# Supplementary material for: Theoretical insights for Improving the Schottky-barrier Height at the Ga$_2$O$_3$/Pt Interface
Source: arXiv:2107.06063 ancillary file (2022-01-05)
Supplement: Supplementary file 1 [file supp.pdf]

# Supplementary Material

## A. $\beta$ -Ga<sub>2</sub>O<sub>3</sub> (100) / H.OH / Pt (111)

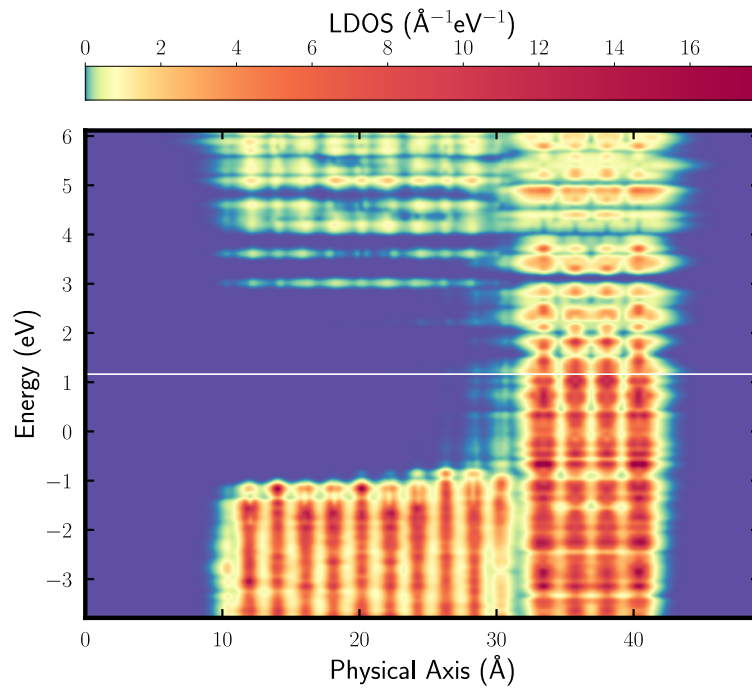

FIG. 1. Local density of states

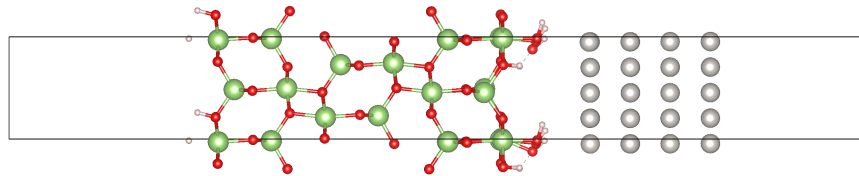

FIG. 2. Relaxed interface structure

B.  $\beta$ -Ga<sub>2</sub>O<sub>3</sub> ( $\bar{2}01$ ) / Pt (111) with reduced strain

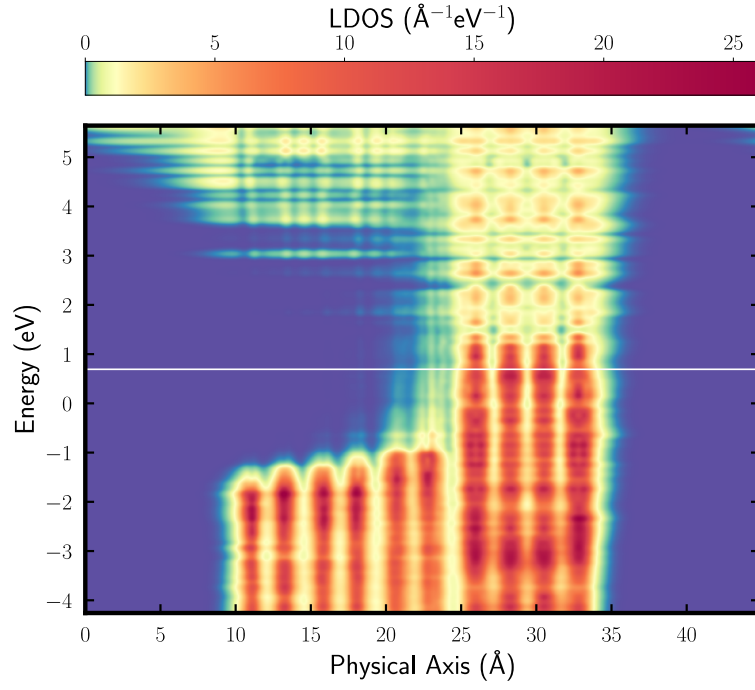

FIG. 3. Local density of states

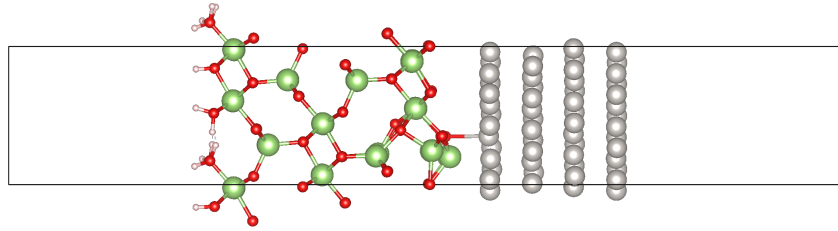

FIG. 4. Relaxed interface structure

C.  $\beta$ -Ga<sub>2</sub>O<sub>3</sub> ( $\bar{2}01$ ) / Pt (221)

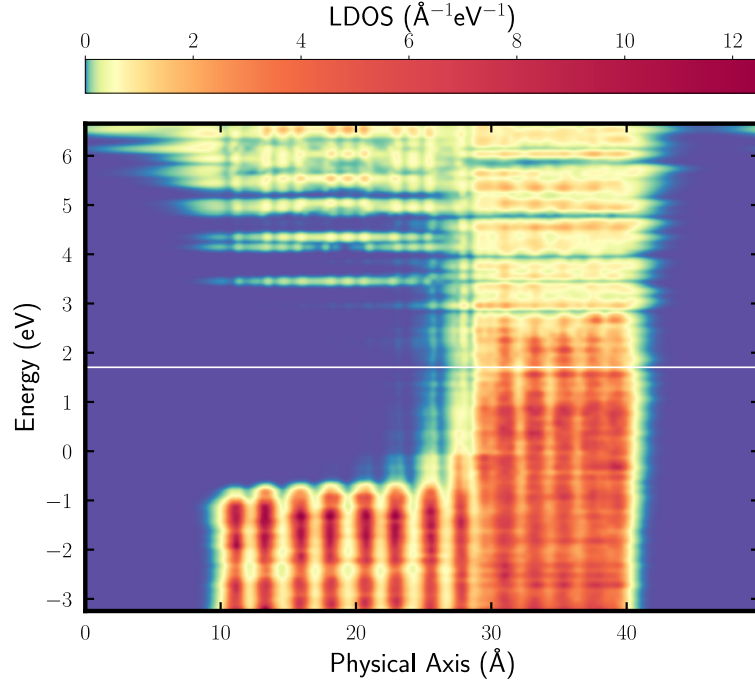

FIG. 5. Local density of states

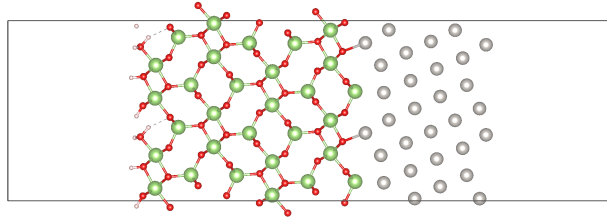

FIG. 6. Relaxed interface structure

D.  $\beta$ -Ga<sub>2</sub>O<sub>3</sub> ( $\bar{2}01$ ) / Pt (321)

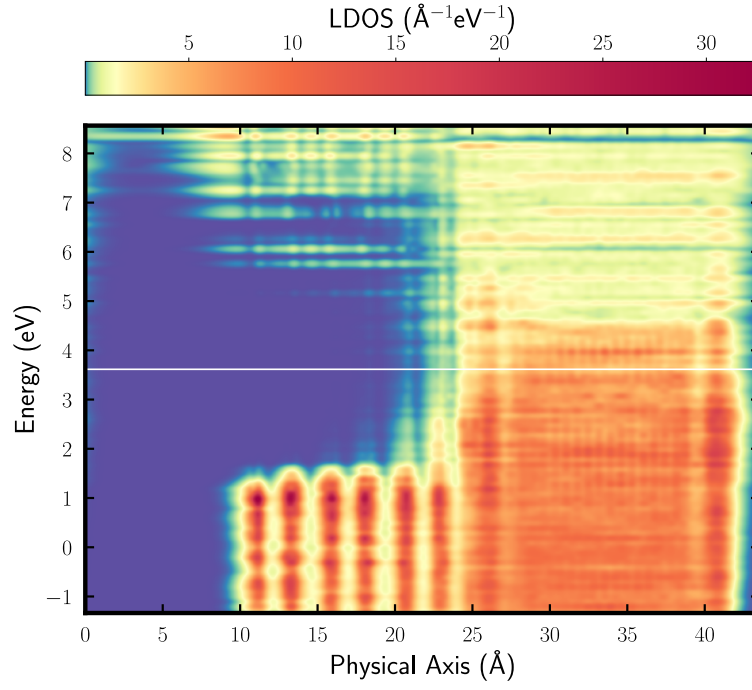

FIG. 7. Local density of states

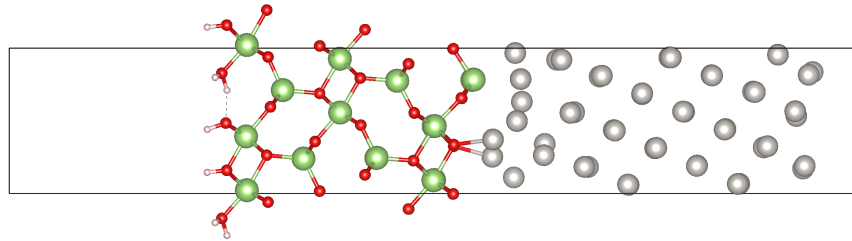

FIG. 8. Relaxed interface structure
